# Supplementary material for: Cycle Flux Ranking of Network Analysis in Quantum Thermal Device
Source: arXiv:2107.07717 source file (2021-07-16)
Supplement: Supplementary file 1 [file supplementary.pdf]

# Supplementary Material:
# Cycle Flux Ranking of Network Analysis in Quantum Thermal Devices

Luqin Wang[1], Zi Wang[1], Chen Wang[2],* and Jie Ren[1]†
[1]*Center for Phononics and Thermal Energy Science, China-EU Joint Center for nanophononics, Shanghai Key Laboratory of Special Artificial Microstructure Materials and Technology, School of Physics Sciences and Engineering, Tongji University, Shanghai 200092, China and*
[2]*Department of Physics, Zhejiang normal University, Jinhua 321004, Zhejiang , P. R. China*
(Dated: July 15, 2021)

This supplementary material exhibits the detail of the two models studied in the main text. In section I, we give a brief introduction of quantum Lindblad master equation, i.e. Eq. (1) in the main text, which has been a standard method in dissipative open quantum systems [1]. Moreover, the general expressions of transition rates are listed in Table I, classified by different types of (either fermionic or bosonic) reservoirs. In section II, we list all the transition rates used in the calculations of the first model: *thermal-drag spin-Seebeck pump*. We give the reasons why cycle $C_1$ and $C_2$ are futile and show the spanning forest rooted on the dominant cycle $C$ which give an explanation of cycle flux via the viewpoint of graph theory. In section III, we list all the transition rates of the *thermal quantum transistor* model. We also draw the cycle trajectories of cycle $C_2$ and $C_3$ which contribute to the transistor effect. Besides, we demonstrate that $C_4$ and $C_5$ compete with cycle $C_6$ and $C_7$, which weaken the NDTC effect.

## I. QUANTUM MASTER EQUATION AND RATE EQUATION

The total Hamiltonian of a dissipative quantum system can always be divided into three parts:

$$H_{tot} = H_s + H_b + V, \tag{S1}$$

which corresponds respectively to the system, reservoir and interaction Hamiltonian. The interaction part provides the channel of energy and particle exchange between quantum system and environment, of which the general form can be formulated as:

$$V = \sum_u A_u \otimes \sum_k (t_{u,k} B_{u,k}). \tag{S2}$$

Here, $A_u$ is the operator of system coupled with the $u$-th reservoir, $B_{u,k}$ is the operator of the $u$-th reservoir with momentum $k$ and $t_{u,k}$ is the coupling strength. Then we define the eigenoperator of $H_s$:

$$A_u(\omega) \equiv \sum_{\varepsilon'-\varepsilon=\omega} \Pi(\varepsilon) A_u \Pi(\varepsilon'), \tag{S3}$$

where $\Pi(\varepsilon)$ is the projection operator which corresponds to the eigenvalue $\varepsilon$. The sum in Eq. S3 is extended over all energy eigenvalue $\varepsilon'$ and $\varepsilon$ of $H_s$ with a fixed energy difference of $\omega$ and $A_u(\omega)$ holds the properties:

$$[H_s, A_u(\omega)] = -\omega A_u(\omega), \tag{S4a}$$
$$[H_s, A_u^\dagger(\omega)] = +\omega A_u^\dagger(\omega), \tag{S4b}$$
$$\sum_\omega A_u(\omega) = A_u. \tag{S4c}$$

Thus the interaction Hamiltonian Eq. S2 becomes:

$$V = \sum_{u,\omega} A_u(\omega) \otimes (\sum_k t_{u,k} B_{u,k}), \tag{S5}$$

In contrast to the closed system, the quantum dynamics of an open system cannot, in general, be represented in terms of a unitary time evolution operator, a quantum master equation. Usually, the Markovian open quantum system obeys a first-order

*Electronic address: wangchenyifang@gmail.com
†Electronic address: Xonics@tongji.edu.cn

linear differential equation for the reduced matrix, $\rho_s(t) = \mathrm{Tr_b}[\rho_s(t)\otimes\rho_b]$, which is known as quantum Markovian master equation in Lindblad form expressed as follows:

$$\frac{d\rho_s(t)}{dt} = i[\rho_s(t), H_s] + \sum_u \mathcal{D}_u[\rho_s(t)], \tag{S6}$$

where the Lindblad superoperator $\mathcal{D}_u[\rho_s(t)] \equiv \Gamma_u(\omega)(A_u(\omega)\rho_s(t)A_u^\dagger(\omega) - \frac{1}{2}\{A_u^\dagger(\omega)A_u(\omega), \rho_s(t)\})$ describes the dissipation induced by $u$-th thermal reservoir. Here, $\{O_1, O_2\} \equiv O_1O_2 + O_2O_1$ denotes the anticomutator. $\Gamma_u$ contains the correlation function of $u$-th bath and the coupling strength:

$$\begin{aligned}\Gamma_u(\omega) &= \int_{-\infty}^{+\infty} d\tau e^{i\omega\tau} \sum_k |t_{u,k}|^2 \langle B_{u,k}^\dagger(\tau)B_{u,k}(0)\rangle \\ &= \sum_k 2\pi|t_{u,k}|^2\delta(\omega-\omega_k)\langle B_{u,k}^\dagger B_{u,k}\rangle \\ &= \mathcal{J}_u(\omega)\langle B_{u,\omega}^\dagger B_{u,\omega}\rangle,\end{aligned} \tag{S7}$$

where $\mathcal{J}_u(\omega) \equiv \sum_k 2\pi|t_{u,k}|^2\delta(\omega-\omega_k)$ is the spectral function of the $u$-th bath. Here we only consider the bath induced quantum transition effects, while ignoring the energy level renormalization effect (Lamb shift, Stark shift).

The reduced density matrix $\rho_s$ can be calculated via the Lindblad master equation S6 and it gives rise to a closed equation of motion for population:

$$P(n,t) = \langle n|\,\rho_s(t)\,|n\rangle \tag{S8}$$

of the eigenstates $|n\rangle$. Hence, the diagonal and the off-diagonal terms decouple in the eigenbasis of $H_s$. According to the quantum master equation, the population is governed by the kinetic equation:

$$\frac{d}{dt}P(n,t) = -\sum_{m\neq n} k_{n,m}P(n,t) + k_{m,n}P(m,t), \tag{S9}$$

which is also known as Pauli master equation. $k_{m,n} \equiv \sum_u k_{u,(m,n)}$ denotes the transition rates from state $|m\rangle$ to $|n\rangle$ contributed by all the reservoirs and the $u$-th reservoir induced component can be expressed as:

$$\begin{aligned}k_{u,(m,n)} &= \Gamma_u(\omega_{m,n})\,\langle m|\,A_u^\dagger\,|n\rangle\,\langle n|\,A_u\,|m\rangle \\ &= \mathcal{J}_u(\omega_{m,n})\langle B_{u,\omega_{m,n}}^\dagger B_{u,\omega_{m,n}}\rangle\,\langle m|\,A_u^\dagger\,|n\rangle\,\langle n|\,A_u\,|m\rangle\,,\end{aligned} \tag{S10}$$

where $\omega_{m,n} = \varepsilon_m - \varepsilon_n$ and $\langle m|\,A_u^\dagger\,|n\rangle = \langle n|\,A_u\,|m\rangle = 1$ in the two systems of this work. Usually, the transition rate can be classified into two types by the coupled bath, Fermionic or Bosonic bath, and in each of them the rate can be divided into two situations, excitation and relaxation process, further. The rates are listed in Table I.

TABLE I: Transition rates coupled with different reservoirs, $\omega > 0$

| | Excitation Process | Relaxation Process |
|---|---|---|
| Fermionic Bath | $\mathcal{J}(\omega)f(\omega,T)$ | $\mathcal{J}(\omega)[1-f(\omega,T)]$ |
| Bosonic Bath | $\mathcal{J}(\omega)N(\omega,T)$ | $\mathcal{J}(\omega)[1+N(\omega,T)]$ |

$f(\omega,T) = \frac{1}{e^{(\omega-\mu)/T}+1}$ is Fermi-Dirac distribution and $N(\omega,T) = \frac{1}{e^{\omega/T}-1}$ is Bose-Einstein distribution with energy $\omega$ and temperature $T$ of the corresponding bath, with the Boltzmann constant set to 1.

## II. DETAILS OF THERMAL-DRAG SPIN-SEEBECK PUMP

For convenience, the six states $\{|0\rangle, |1\rangle\} \otimes \{|0\rangle, |\uparrow\rangle, |\downarrow\rangle\}$ in main text are simplified by the Arabic numerals and shown in follows:

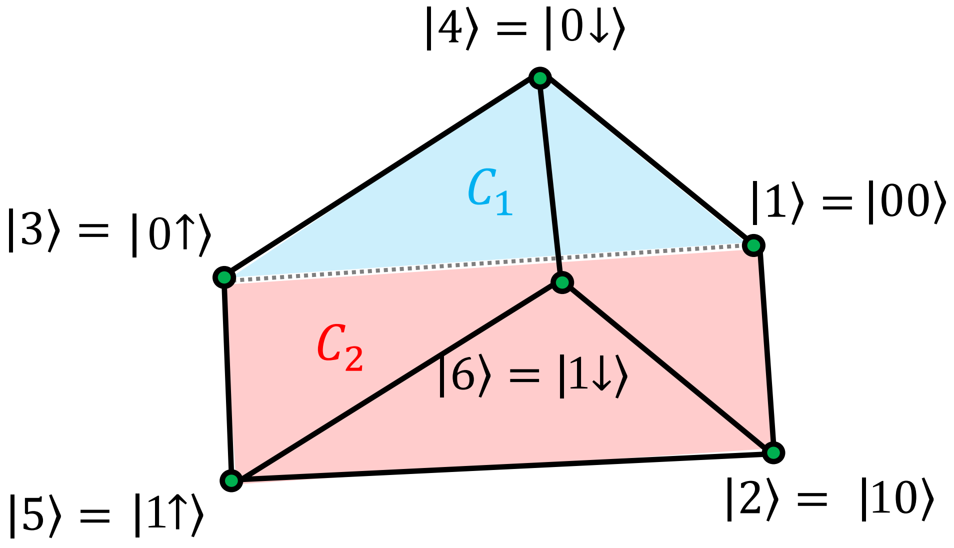


FIG. S1: Quantum transition network of *thermal-drag spin-Seebeck pump* with simplified notations of the six states. Cycle trajectories of $C_1$ and $C_2$ are emphasized by the blue and red shadow areas, respectively.

With the help of Table I, all the transition rates are listed in the following table:

TABLE II: Transition Rates

| | |
|---|---|
| $k_{1,2} = \mathcal{J}_1(\omega_{2,1})f(\omega_{2,1},T_1) + \mathcal{J}_2(\omega_{2,1})f(\omega_{2,1},T_2)$ | $k_{2,1} = \mathcal{J}_1(\omega_{2,1})[1-f(\omega_{2,1},T_1)] + \mathcal{J}_2(\omega_{2,1})[1-f(\omega_{2,1},T_2)]$ |
| $k_{1,3} = \mathcal{J}_3(\omega_{3,1})f(\omega_{3,1},T_3)$ | $k_{3,1} = \mathcal{J}_3(\omega_{3,1})[1-f(\omega_{3,1},T_3)]$ |
| $k_{1,4} = \mathcal{J}_3(\omega_{4,1})f(\omega_{4,1},T_3)$ | $k_{4,1} = \mathcal{J}_3(\omega_{4,1})[1-f(\omega_{4,1},T_3)]$ |
| $k_{2,5} = \mathcal{J}_3(\omega_{5,2})f(\omega_{5,2},T_3)$ | $k_{5,2} = \mathcal{J}_3(\omega_{5,2})[1-f(\omega_{5,2},T_3)]$ |
| $k_{2,6} = \mathcal{J}_3(\omega_{6,2})f(\omega_{6,2},T_3)$ | $k_{6,2} = \mathcal{J}_3(\omega_{6,2})[1-f(\omega_{6,2},T_3)]$ |
| $k_{3,4} = \mathcal{J}_4(\omega_{4,3})N(\omega_{4,3},T_4)$ | $k_{4,3} = \mathcal{J}_4(\omega_{4,3})[1+N(\omega_{4,3},T_4)]$ |
| $k_{3,5} = \mathcal{J}_1(\omega_{5,3})f(\omega_{5,3},T_1) + \mathcal{J}_2(\omega_{5,3})f(\omega_{5,3},T_2)$ | $k_{5,3} = \mathcal{J}_1(\omega_{5,3})[1-f(\omega_{5,3},T_1)] + \mathcal{J}_2(\omega_{5,3})[1-f(\omega_{5,3},T_2)]$ |
| $k_{4,6} = \mathcal{J}_1(\omega_{6,4})f(\omega_{6,4},T_1) + \mathcal{J}_2(\omega_{6,4})f(\omega_{6,4},T_2)]$ | $k_{6,4} = \mathcal{J}_2(\omega_{6,4})[1-f(\omega_{6,4},T_1)] + \mathcal{J}_2(\omega_{6,4})[1-f(\omega_{6,4},T_2)]$ |
| $k_{5,6} = \mathcal{J}_4(\omega_{6,5})N(\omega_{6,5},T_4)$ | $k_{6,5} = \mathcal{J}_4(\omega_{6,5})[1+N(\omega_{6,5},T_4)]$ |

Here, $\omega_{i,j}$ is the energy level difference which can be defined as $\omega_{i,j} \equiv \omega_i - \omega_j$. And $J_u(\omega)$ is the spectral function of the $u$-th bath. Without losing generality, the spectral functions in the wide band limit are used here [2]: $\mathcal{J}_u(\omega) = 0.1$, $u = \{1,2,3,4\}$.

The positive spin current $I_3$ and $I_4$ are defined as the spin flows into the lower subsystem per unit time from the spinful electron and magnon bath respectively, and they can be formulated as following:

$$I_3 \equiv -\frac{i}{2}\langle[H_{tot}, \sum_k (c^\dagger_{L\uparrow,k}c_{L\uparrow,k} - c^\dagger_{L\downarrow,k}c_{L\downarrow,k})]\rangle, \tag{S11a}$$

$$I_4 \equiv -i\langle[H_{tot}, \sum_q b^\dagger_q b_q]\rangle, \tag{S11b}$$

where $c^\dagger_{L\sigma,k}(c_{L\sigma,k})$ is the create(annihilation) operator in spinful electron reservoir with spin $\sigma$ and momentum $k$, and $b^\dagger_q(b_q)$ is the create(annihilation) operator in magnon reservoir with momentum $q$. Here we use the fact that an electron (magnon) has a quantized spin $\frac{1}{2}$ (-1) with $\hbar$ set to 1. And the positive electron current $J_1$ and $J_2$ can be similarly defined as the electron flows into the upper quantum dot per unit time with the formula form:

$$J_1 \equiv -\frac{i}{\hbar}\langle[H_{tot}, \sum_k c^\dagger_{U1,k}c_{U1,k}]\rangle, \tag{S12a}$$

$$J_2 \equiv -\frac{i}{\hbar}\langle[H_{tot}, \sum_k c^\dagger_{U2,k}c_{U2,k}]\rangle, \tag{S12b}$$

where $c^\dagger_{U1,k}$ $(c_{U1,k})$ and $c^\dagger_{U2,k}$ $(c_{U2,k})$ are the creation (annihilation) operator in 1-st and 2-nd spinless electron reservoir, respectively.

For cycle flux analysis of spin (heat) current, we rank 28 cycle fluxes and partially show them in the Fig. 2(e) of the main text. Before analyzing the spanning trees of dominant cycle $C$, we first give a reason why we ignore the top 2 ranked paired cycles. The top bidirectional cycles is: $C_1$ : $|00\rangle$ $(|1\rangle) \leftrightarrow |0\downarrow\rangle$ $(|4\rangle) \leftrightarrow |0\uparrow\rangle$ $(|3\rangle) \leftrightarrow |00\rangle$ $(|1\rangle)$ whose cycle fluxes are largest. But the clockwise and anti-clockwise counterparts completely cancel with each other,

$$\frac{k_{1,3}k_{3,4}k_{4,1}}{k_{3,1}k_{4,2}k_{1,4}} = e^{\frac{\varepsilon_{L\uparrow}}{T_L}} e^{\frac{\varepsilon_{L\downarrow}-\varepsilon_{L\uparrow}}{T_L}} e^{\frac{-\varepsilon_{L\downarrow}}{T_L}} = 1, \tag{S13}$$

which implies the clockwise and anti-clockwise component of cycle $C_1$ satisfy the detailed balance. Thus $C_1$ makes no contribution to the spin current. The second-ranked paired cycles $C_2$ : $|00\rangle \leftrightarrow |0\uparrow\rangle \leftrightarrow |1\uparrow\rangle \leftrightarrow |10\rangle \leftrightarrow |00\rangle$ is futile because the spin state of lower dot keeps unchanged during the cyclic process. Hence these two paired cycles are not the dominant cycles for spin pump and we identify the next paired cycles $C$ dominate the *thermal-drag spin-Seebeck pump*.

Spanning tree is defined as a tree which is a connected directed or undirected graph with no cycles. And if a tree has one vertex $d$ which is the drain of all its incident edges, this tree is called the tree rooted on $d$. Then all the spanning trees (spanning forest) rooted on the dominant cycle $C$ are shown in Fig. S2 (a), (b) and (c). Each of them represents a dynamical process that the state transfers into another state contained in the dominant cycle $C$. For example, when the system is in $|6\rangle$ $(|1\downarrow\rangle)$, the lower quantum dot emits a magnon(whose spin is -$\hbar$) to the magnon bath, while the state transfers to $|5\rangle$ $(|1\uparrow\rangle)$ illustrated in Fig. S2 (a), with the transition rate $k_{6,5}$. The Laplacian matrix in this model is express as:

$$L = \begin{pmatrix} \sum_{j\neq 1} k_{1,j} & -k_{2,1} & -k_{3,1} & -k_{4,1} & 0 & 0 \\ -k_{1,2} & \sum_{j\neq 2} k_{2,j} & 0 & 0 & -k_{5,2} & -k_{6,2} \\ -k_{1,3} & 0 & \sum_{j\neq 3} k_{3,j} & -k_{4,3} & -k_{5,3} & 0 \\ -k_{1,4} & 0 & -k_{3,4} & \sum_{j\neq 4} k_{4,j} & 0 & -k_{6,4} \\ 0 & -k_{2,5} & -k_{3,5} & 0 & \sum_{j\neq 5} k_{5,j} & -k_{6,5} \\ 0 & -k_{2,6} & 0 & -k_{4,6} & -k_{5,6} & \sum_{j\neq 6} k_{6,j} \end{pmatrix}. \tag{S14}$$

Thus we can get $det(L[C;C]) = \sum_{j\neq 6} k_{6,j} = k_{6,2} + k_{6,4} + k_{6,5}$, where $L[C;C]$ is the matrix obtained by deleting from $L$ the rows and columns corresponding to the states in cycle $C$. $det(L[C;C])$ describes the quantum transition process illustrated in Fig. S2 (a) (b) (c) respectively and is summarized in Fig. S2(d). The transition process of the Fig. S2(d), $det(L[C;C])$, is identical to shrinking the dominant cycle $C$ into a new vertex $d$ shown in Fig. S2(e). This effective Laplacian matrix is expressed as:

$$L' = \begin{pmatrix} k_{d,6} & -k_{6,d} \\ -k_{d,6} & k_{6,d} \end{pmatrix} = \begin{pmatrix} k_{2,6} + k_{4,6} + k_{5,6} & -k_{6,2} - k_{6,4} - k_{6,5} \\ -k_{2,6} - k_{4,6} - k_{5,6} & k_{6,2} + k_{6,4} + k_{6,5} \end{pmatrix}. \tag{S15}$$

Deleting the first row and first column in $L'$, we can get $det(L'[1;1]) = k_{6,2} + k_{6,4} + k_{6,5}$ which is same with $det(L[C;C])$.

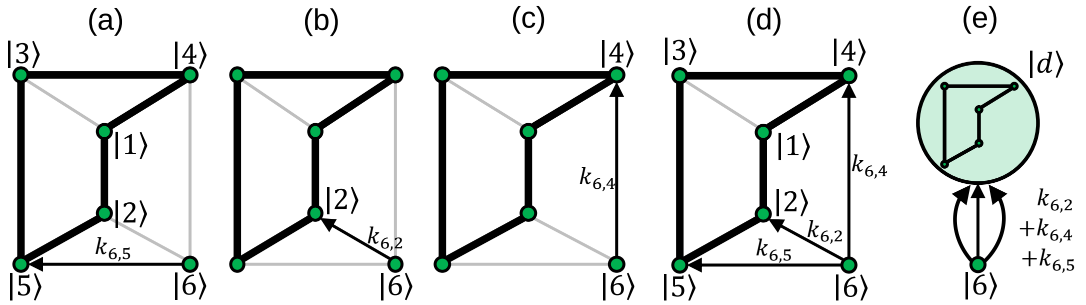


FIG. S2: **Spanning trees rooted on cycle** $C$**.** (a) (b) (c) are all the spanning trees rooted on the dominant cycle $C$. (d) The transition graph corresponding to the $det(L[C;C])$ is equivalent to a new graph with shrinking the dominant cycle $C$ into a new vertex $d$ shown in (e), where the big green circle denote the new vertex $d$.

## III. DETAILS OF QUANTUM THERMAL TRANSISTOR

In this *quantum thermal transistor* model, we use five Ohmic spectral functions [3] with different coupling strengths [4]:

$$J_{L,+}(\omega) = J_{R,+}(\omega) = 0.004\omega, \tag{S16a}$$
$$J_{L,-}(\omega) = J_{R,-}(\omega) = 0.003\omega, \tag{S16b}$$
$$J_M(\omega) = 0.001\omega. \tag{S16c}$$

Different spectral functions will not qualitatively change the transport behaviors, and the cycle flux method is still powerful to analyze this kind of complex quantum system. And for convenience, the eighteen states in main text $\{|G\rangle, |+\rangle, |-\rangle\}otimes\{|\uparrow\rangle, |\downarrow\rangle\} \otimes \{|G\rangle, |+\rangle, |-\rangle\}$ are simplified by the Arabic numerals and shown in follows:

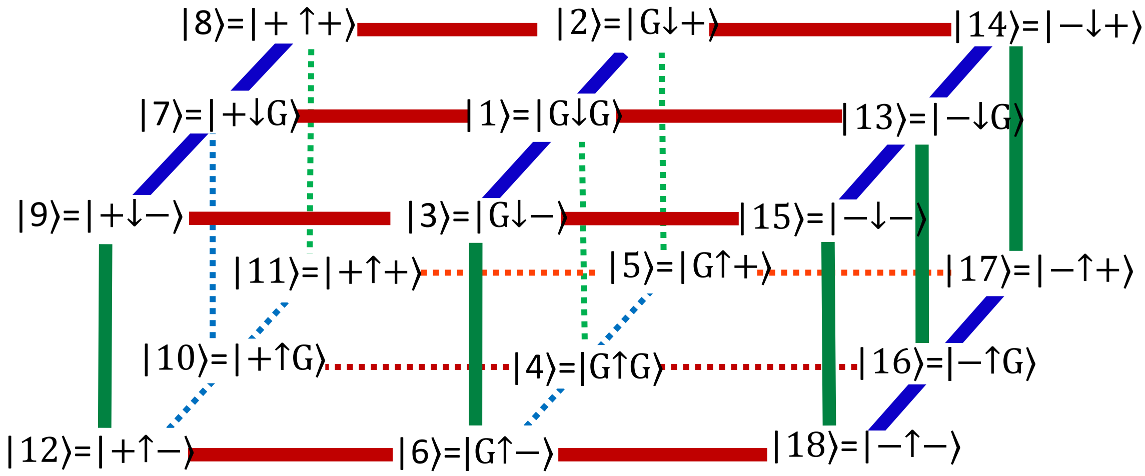


FIG. S3: Quantum transition network of *quantum thermal transistor* model with simplified notations of the eighteen states.

The transition rates are expressed as follows:

TABLE III: Transition Rate

| | |
|---|---|
| $k_{1,2} = J_{R,+}(\omega_{2,1})N(\omega_{2,1}, T_R)$ | $k_{2,1} = J_{R,+}(\omega_{2,1})[1 + N(\omega_{2,1}, T_R)]$ |
| $k_{1,3} = J_{R,-}(\omega_{3,1})N(\omega_{3,1}, T_R)$ | $k_{3,1} = J_{R,+}(\omega_{3,1})[1 + N(\omega_{3,1}, T_R)]$ |
| $k_{1,4} = J_M(\omega_{4,1})N(\omega_{4,1}, T_M)$ | $k_{4,1} = J_M(\omega_{4,1})[1 + N(\omega_{4,1}, T_M)]$ |
| $k_{1,7} = J_M(\omega_{7,1})N(\omega_{7,1}, T_M)$ | $k_{7,1} = J_M(\omega_{7,1})[1 + N(\omega_{7,1}, T_M)]$ |
| $k_{1,13} = J_{L,-}(\omega_{13,1})N(\omega_{13,1}, T_L)$ | $k_{13,1} = J_{L,-}(\omega_{13,1})[1 + N(\omega_{13,1}, T_L)]$ |
| $k_{2,5} = J_M(\omega_{5,2})N(\omega_{5,2}, T_M)$ | $k_{5,2} = J_M(\omega_{5,2})[1 + N(\omega_{5,2}, T_M)]$ |
| $k_{2,8} = J_{L,+}(\omega_{8,2})N(\omega_{8,2}, T_L)$ | $k_{8,2} = J_{L,+}(\omega_{8,2})[1 + N(\omega_{8,2}, T_L)]$ |
| $k_{2,14} = J_{L,-}(\omega_{14,2})N(\omega_{14,2}, T_L)$ | $k_{14,2} = J_{L,-}(\omega_{14,2})[1 + N(\omega_{14,2}, T_L)]$ |
| $k_{3,6} = J_M(\omega_{6,3})N(\omega_{6,3}, T_M)$ | $k_{6,3} = J_M(\omega_{6,3})[1 + N(\omega_{6,3}, T_M)]$ |
| $k_{3,9} = J_{L+}(\omega_{9,3})N(\omega_{9,3}, T_L)$ | $k_{9,3} = J_{L+}(\omega_{9,3})[1 + N(\omega_{9,3}, T_L)]$ |
| $k_{3,15} = J_{L-}\omega_{15,3}N(\omega_{15,3}, T_L)$ | $k_{15,3} = J_{L-}\omega_{15,3}[1 + N(\omega_{15,3}, T_L)]$ |
| $k_{4,5} = J_{R+}(\omega_{5,4})N(\omega_{5,4}, T_R)$ | $k_{5,4} = J_{R+}(\omega_{5,4})[1 + N(\omega_{5,4}, T_R)]$ |
| $k_{4,6} = J_{R-}(\omega_{6,4})N(\omega_{6,4}, T_R)$ | $k_{6,4} = J_{R-}(\omega_{6,4})[1 + N(\omega_{6,4}, T_R)]$ |
| $k_{4,10} = J_{L+}(\omega_{10,4})N(\omega_{10,4}, T_L)$ | $k_{10,4} = J_{L+}(\omega_{10,4})[1 + N(\omega_{10,4}, T_L)]$ |
| $k_{4,16} = J_{L-}(\omega_{16,4})N(\omega_{16,4}, T_L)$ | $k_{16,4} = J_{L-}(\omega_{16,4})[1 + N(\omega_{16,4}, T_L)]$ |
| $k_{5,11} = J_{L+}(\omega_{11,5})N(\omega_{11,5}, T_L)$ | $k_{11,5} = J_{L+}(\omega_{11,5})[1 + N(\omega_{11,5}, T_L)]$ |
| $k_{5,17} = J_{L-}(\omega_{17,5})N(\omega_{17,5}, T_L)$ | $k_{17,5} = J_{L-}(\omega_{17,5})[1 + N(\omega_{17,5}, T_L)]$ |
| $k_{6,12} = J_{L+}(\omega_{12,6})N(\omega_{12,6}, T_L)$ | $k_{12,6} = J_{L+}(\omega_{12,6})[1 + N(\omega_{12,6}, T_L)]$ |
| $k_{6,18} = J_{L-}\omega_{18,6}N(\omega_{18,6}, T_L)$ | $k_{18,6} = J_{L-}\omega_{18,6}[1 + N(\omega_{18,6}, T_L)]$ |
| $k_{7,8} = J_{R+}(\omega_{8,7})N(\omega_{8,7}, T_R)$ | $k_{8,7} = J_{R+}(\omega_{8,7})[1 + N(\omega_{8,7}, T_R)]$ |
| $k_{7,9} = J_{R-}(\omega_{9,7})N(\omega_{9,7}, T_R)$ | $k_{9,7} = J_{R-}(\omega_{9,7})[1 + N(\omega_{9,7}, T_R)]$ |
| $k_{7,10} = J_M(\omega_{10,7})N(\omega_{10,7}, T_M)$ | $k_{10,7} = J_M(\omega_{10,7})[1 + N(\omega_{10,7}, T_M)]$ |
| $k_{8,11} = J_M(\omega_{11,8})N(\omega_{11,8}, T_M)$ | $k_{11,8} = J_M(\omega_{11,8}[1 + N(\omega_{11,8}, T_M)]$ |
| $k_{9,12} = J_M(\omega_{12,9})N(\omega_{12,9}, T_M)$ | $k_{12,9} = J_M(\omega_{12,9})[1 + N(\omega_{12,9}, T_M)]$ |
| $k_{10,11} = J_{R+}(\omega_{11,10})N(\omega_{11,10}, T_R)$ | $k_{11,10} = J_{R+}(\omega_{11,10})[1 + N(\omega_{11,10}, T_R)]$ |
| $k_{10,12} = J_{R-}(\omega_{12,10})N(\omega_{12,10}, T_R)$ | $k_{12,10} = J_{R-}(\omega_{12,10})[1 + N(\omega_{12,10}, T_R)]$ |
| $K_{13,14} = J_{R+}(\omega_{14,13})N(\omega_{14,13}, T_R)$ | $K_{14,13} = J_{R+}(\omega_{14,13})[1 + N(\omega_{14,13}, T_R)]$ |
| $k_{13,15} = J_{R-}(\omega_{15,13})N(\omega_{15,13}, T_R)$ | $k_{15,13} = J_{R-}(\omega_{15,13})[1 + N(\omega_{15,13}, T_R)]$ |
| $k_{13,16} = J_M(\omega_{16,13})N(\omega_{16,13}, T_M)$ | $k_{16,13} = J_M(\omega_{16,13})[1 + N(\omega_{16,13}, T_M)]$ |
| $k_{14,17} = J_M(\omega_{17,14})N(\omega_{17,14}, T_M)$ | $k_{17,14} = J_M(\omega_{17,14})[1 + N(\omega_{17,14}, T_M)]$ |
| $k_{15,18} = J_M(\omega_{18,15})N(\omega_{18,15}, T_M)$ | $k_{18,15} = J_M(\omega_{18,15})[1 + N(\omega_{18,15}, T_M)]$ |
| $k_{16,17} = J_{R+}(\omega_{17,16})N(\omega_{16,17}, T_R)$ | $k_{17,16} = J_{R+}(\omega_{17,16})[1 + N(\omega_{16,17}, T_R)]$ |
| $k_{16,18} = J_{R-}(\omega_{18,16})N(\omega_{18,16}, T_R)$ | $k_{18,16} = J_{R-}(\omega_{18,16})[1 + N(\omega_{18,16}, T_R)]$ |

$k_{i,j}$ is the transition rate from state $|i\rangle$ to state $|j\rangle$. And $N(\omega, T) = \frac{1}{e^{\omega/T}-1}$ is Bose-Einstein distribution with energy $\omega$ and temperature $T$ of the corresponding bath.

Besides the dominant cycle $C_1$, other top-ranked cycles also contribute to the transistor behaviors. These behaviors are governed by not only the relative dominant cycle, but also other comparable top-ranked cycles. This could be an analogy of Taylor expansion in which the dominant cycle is the first order term and other top-ranked cycles are high order terms which depict the more detailed information of the function. The cycle trajectories of $C_2$ and $C_3$ is drawn in Fig. S4. It is easy to identify that $C_2$ and $C_3$ have two similar properties with the dominant cycle $C_1$. One is $C_2$ and $C_3$ do no contributions to $J_M$ due to $\omega_{9,12} + \omega_{17,14} = 0$ which is same with cycle $C_1$. The other property is entirely pumping heat from the left reservoir to the right reservoir. In cycle $C_2$, the total energy extracted from left reservoir is $\omega_{6,18} + \omega_{12,6} + \omega_{1,7} + \omega_{14,2} = 20 > 0$, and the total energy pumped into right reservoir is $\omega_{9,7} + \omega_{1,2} + \omega_{17,16} + \omega_{16,18} = 20 > 0$. In cycle $C_3$, the total energy extracted from left reservoir is $\omega_{12,6} + \omega_{2,8} + \omega_{14,2} + \omega_{4,16} = 20 > 0$, and the total energy pumped into right reservoir is $\omega_{9,7} + \omega_{7,8} + \omega_{17,16} + \omega_{4,6} = 20 > 0$. Thus $C_2$ and $C_3$ together assist $C_1$ to build the thermal quantum transistor and switch effect.

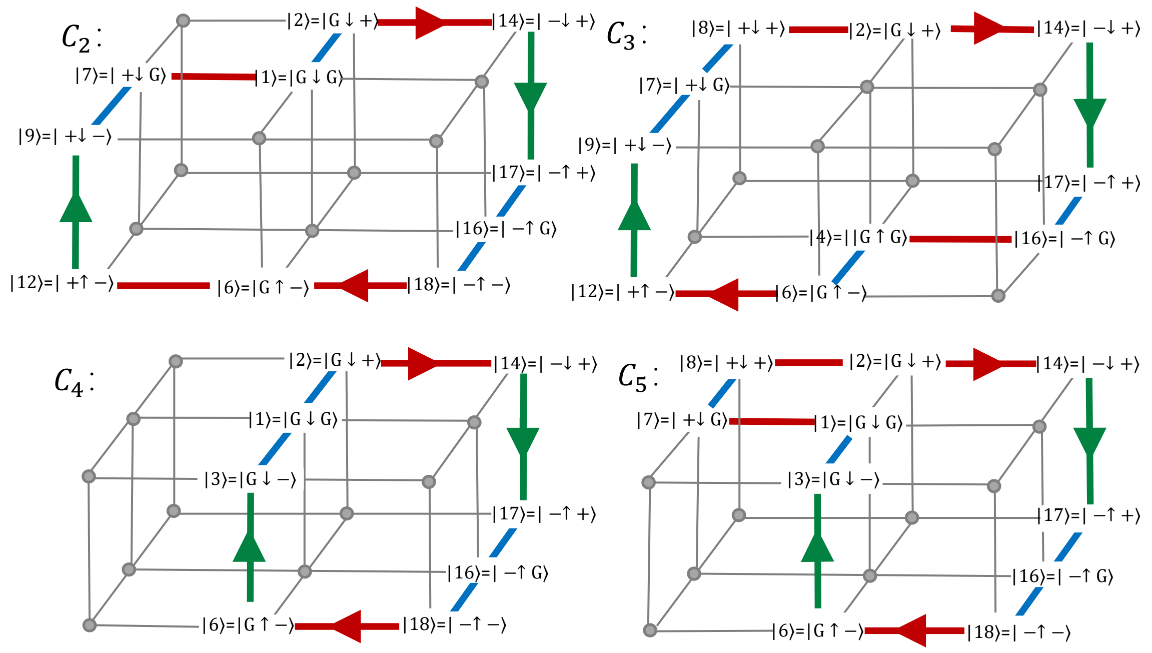


FIG. S4: Cycle trajectories of $C_2$, $C_3$, $C_4$, $C_5$. The red, green and blue lines indicate the transitions induced by left, middle and right bath, respectively.

The values of $J_{C_4}$ and $J_{C_5}$ are the same which cannot be distinguished, thus we represent them by one line in Fig.3 (d) of main text. In the current parameters, $|G\downarrow G\rangle \to |G\downarrow +\rangle$ in cycle $C_4$ is an equivalent shortcut to $|G\downarrow G\rangle \to |+\downarrow G\rangle \to |+\downarrow +\rangle \to |G\downarrow +\rangle$ in cycle $C_5$. During the cyclic processes of $C_4$ and $C_5$, the middle two-level subsystem pumps heat current into system from the middle bath, $\omega_{3,6} + \omega_{17,14} = 10 > 0$, which will weaken NDTC effect. With the opening of channels $C_4$ and $C_5$ caused by the increasing $T_M$, they together compete with $C_6$ and $C_7$. Thus $J_M$ trends to be positive in higher $T_M$ and the NDTC effect transforms to the normal PDTC effect.

[1] H.-P. Breuer, F. Petruccione, et al., *The theory of open quantum systems* (Oxford University Press on Demand, 2002).
[2] B. Sothmann and M. Bttiker, EPL (Europhysics Letters) **99**, 27001 (2012), URL https://doi.org/10.1209/0295-5075/99/27001.
[3] K. Joulain, J. Drevillon, Y. Ezzahri, and J. Ordonez-Miranda, Phys. Rev. Lett. **116**, 200601 (2016), URL https://link.aps.org/doi/10.1103/PhysRevLett.116.200601.
[4] S.-W. Li, C. Cai, and C. Sun, Annals of Physics **360**, 19 (2015), ISSN 0003-4916, URL https://www.sciencedirect.com/science/article/pii/S0003491615001888.
